# Supplementary material for: Exploring the Landscape of Distributed Graph Sketching
Source: arXiv:2410.07518 source file (2024-11-15)
Supplement: Supplementary file 1 [file pht_design.tex]

\section{\Treename Design Considerations}
\label{app:pipeline_design}
To avoid the performance detriments of cascading flushes, in which a flush triggers another flush of one of its children, we implement optimizations inspired by the work in~\cite{BenderDaFa20Flushing}. Cascading flushes (and flushes to leaves in general) are particularly expensive for this problem; The latency difference between accessing the root nodes (which are likely stored in L1 or L2) and the leaf nodes (which are likely stored in RAM) is approximately a factor of 20-80\cite{Brett16}. Specifically, at each subsequent thread-local level of the DAG the buffer size and fan-out are both doubled. This double-doubling means that, in expectation, when we flush a root node, we flush $\frac{1}{4}$ level two nodes, $\frac{1}{16}$ level three nodes, etc. It also helps these buffers fit into the different levels of cache; our tree grows approximately as fast as cache does. This dramatically improves the latency of each \treename root flush as we no longer flush an entire root-to-leaf path in expectation. Our implementation uses $5$ total levels, $3$ of which are thread-local. The $5$th level are called leaf buffers and are treated as a special case; there are $V$ buffers, each of size $O(\alpha\log^2\nodesize)$.
