# Supplementary material for: Exploring the Landscape of Distributed Graph Sketching
Source: arXiv:2410.07518 source file (2024-11-15)
Supplement: Supplementary file 2 [file prior_connectivity.tex]

\section{Prior Work in Connectivity Sketching}
\label{app:alg}

We summarize \algname and \graphzep, respectively Ahn \etal's~\cite{Ahn2012} and Tench \etal's~\cite{graphzeppelin} semi-streaming algorithms for computing a spanning forest (and therefore the connected components) of a graph.  These algorithms have some overlap so for conciseness we describe them in parallel and note where they differ.

For each vertex $v_i$ in $G$, define the \defn{characteristic vector} $\charvec_i$ of $v_i$ to be an $\binom{n}{2}$-dimensional vector indexed by the set of possible edges in $\graph$.  $\charvec_i[(j,k)]$ is only nonzero when $i = j$ or $i = k$ and edge $(j,k) \in \edges$.  That is, $\charvec_i \in \{-1,0,1\}^{\binom{\nodesize}{2}}$ s.t. for all $0 \leq j < k < {\binom{\nodesize}{2}}$: 
$$\charvec_i[(j,k)] = \left\{ \begin{array}{ll}
            1 & \quad i = j \text{ and }(v_j, v_k) \in \edges \\
            -1 & \quad i = k \text{ and }(v_j, v_k) \in \edges \\
            0 & \quad \text{otherwise} 
            
        \end{array}\right\}%\{1$ $if$ $i = j$ $and$ $(v_j, v_k) \in E, -1$ $if$ $i = k$ $and$ $(v_j, v_k) \in E, 0 \text{ otherwise}\}
$$

%The characteristic vector $a_i$ is a 1-dimensional vector indexed by the set of possible edges in $\graph$.  $a_i[(j,k)]$ is only nonzero when $i = j$ or $i = k$ and edge $(j,k) \in \edges$.

These characteristic vectors have an important property that is vital for computing connectivity: For any $S \subset \nodes$, the sum of the characteristic vectors of the vertices in $S$ is a direct encoding of the edges across the cut $(S, \nodes \setminus S$).  That is, let $x = \sum_{v \in S} \charvec_v$ and then % $x\in \{-1,0,1\}^{\binom{n}{2}}$ and 
$|x[(j,k)]| = 1$ iff $(j,k) \in E(S, \nodes \setminus S)$.

It is simple to update the characteristic vectors as stream updates arrive. Initialize $\charvec_i = \{0\}^{\binom{\nodesize}{2}}$ for all $i$. For each stream update $s = ((u,v), \Delta)$, set $\charvec_u[u,v] += \Delta$ and $\charvec_v[u,v] += -\Delta$.Using these vectors, we immediately have a (very inefficient) algorithm for computing the connected components from a stream by running Boruvka's algorithm~\cite{boruvka} for finding a spanning forest as follows.  For the first round of the algorithm, from each $a_i$ arbitrarily choose one nonzero entry $(w,y)$ (an edge in $\edges$ s.t. w = i or y = i).  Add $e_i$ to the spanning forest.  For each connected component $C$ in the spanning forest, compute the characteristic vector of $C$: $\charvec_C = \sum_{v\in C} \charvec_v$.  Proceed similarly for the remaining rounds of Boruvka's algorithm: in each round, choose one nonzero entry from the characteristic vector of each connected component and add the corresponding edges to the spanning forest.  Sum the characteristic vectors of the component vertices of the connected components in the spanning forest. Repeat until no new merges are possible.  This takes at most $\log(\nodesize)$ rounds.

The key idea to make this a small-space algorithm is to use $\ell_0$-sampling ~\cite{l0sketch} to run this version of Boruvka's algorithm by compressing each characteristic vector $\charvec_i$ into a data structure of size $O(\log^2(\nodesize))$ that can return a nonzero entry of $\charvec_i$ with high probability.  For all $\ell_0$ samplers discussed in this paper, $\sketch(\charvec)$ is a vector and adding two sketches is equivalent to adding their vectors elementwise. The $\ell_0$ sampler may fail to sample an element; for Boruvka's algorithm to succeed in $O(\log\nodesize)$ rounds, each sampler must fail with at most constant probability.

\algname uses an $\ell_0$ sampler of Cormode \etal:

\begin{theorem} (Adapted from ~\cite{l0sketch}, Theorem 1):
Given a 2-wise independent hash family $\mathcal{F}$ and an input vector $x \in \mathbb{Z}^n$, there is an $\ell_0$-sampler using $O(\log^2(n)\log(1/\delta))$ space that succeeds with probability at least $1 - \delta$.
\end{theorem}

\graphzep uses \cubesketch, an $\ell_0$ sampler that is purpose-built for sketching characteristic vectors and as a result reduces average-case update cost:

\cubesketchthm*

%\david{clarify support finding only?}
\sysname uses a new, improved $\ell_0$ sampler which we call \sketchname which improves worst-case update time to $O(\log(n))$ and reduces space by a constant factor. It supports the same operations as \cubesketch and is used to run Boruvka in the same way. We summarize \cubesketch and present \sketchname in Section~\ref{subsec:cameo}. 
%we choose to use \cubesketch for $\ell_0$ sampling because it performs better in practice~\cite{graphzeppelin}.\david{now we say we use our own thing which is better than cubesketch}

We denote the $\ell_0$ sketch of a vector $x$ as $\sketch(x)$.  Since the sketch is linear, $\sketch(x) + \sketch(y) = \sketch(x+y)$ for any vectors $x$ and $y$.  This allows us to process stream updates as follows: we maintain a running sum of the sketches of each stream update, which is equivalent to a sketch of the vector defined by the stream. That is, let $\charvec_i^t$ denote $\charvec_i$ after stream prefix $\stream_t$. For the $j$th stream update $\streamelement_j = ((i,x),\Delta)$ we obtain $\sketch(\charvec_i^j) = \sketch(\streamelement_j) + \sketch(\charvec_i^{j-1})$. For each stream update $\streamelement_j$, \algname computes $\sketch(\charvec_i^j)$ as soon as $\streamelement_j$ arrives from the input stream. In contrast, \graphzep inserts $\streamelement_j$ into a \defn{gutter tree} of size $O(\nodesize \log^3(\nodesize))$ that write-efficiently collects updates by endpoint. When $O(\log^3(\nodesize))$ updates have been collected for vertex $i$, $\streamelement_j$ and all other collected updates for vertex $i$ are added to $\sketch(\charvec_i)$. The gutter tree allows stream ingestion to be done I/O optimally when the gutter tree and sketches are stored on disk; we omit the details here.
mark
Linearity also allows Ahn \etal to emulate the merging step of Boruvka's algorithm by summing the sketches of all vertices in each connected component.  They require $\log\nodesize)$ independent $\ell_0$ sketches for each $v \in \nodes$, one for each round\footnote{Ahn \etal~\cite{Ahn2012} the authors note that adaptivity concerns require the use of new sketches for each round of Boruvka's algorithm.}, so the size of the sketch data structure for each vertex is $O(\log^3\nodesize)$.  We refer to the sketch data structure for each vertex as a \defn{vertex sketch} and each of its $\log\nodesize$ $\ell_0$-subsketches as \cubesketch{}s. Since \graphzep is designed to run efficiently out-of-core, it modifies this iterated vertex merging process to be write-optimal~\cite{graphzeppelin}; we omit the details here because \sysname does not use this technique.

The total size of the entire sketch data structure for either algorithm is $O\nodesize \log^3(\nodesize)$. \graphzep's gutter tree structure also has size $O(\nodesize \log^3\nodesize)$. Recent work ~\cite{nelson2019optimal} has shown that this space is asymptotically optimal. Because their $\ell_0$ sketch algorithms are randomized and can sometimes fail, the connectivity algorithm may also fail (subject to the choice of randomness used for the sketches). However, they show that these algorithms succeed with high probability: \ie they fail to return the correct answer with probability at most $1/\nodesize^c$ for some constant $c\geq1$ ($c$ appears as a constant factor in the space).
