# Supplementary material for: Exploring the Landscape of Distributed Graph Sketching
Source: arXiv:2410.07518 source file (2024-11-15)
Supplement: Supplementary file 3 [file rounds.tex]

\section{\sketchname Experiment}
\label{app:rounds}

We experimentally confirm that our implementation of \sketchname achieves the success probability proved in Lemma~\ref{lem:7-wise-sketch}. 
The experiment is as follows: 
\begin{enumerate}
    \item We initialize an empty \sketchname column $C$ with a unique seed for a vector of length $n=2^{24}$
    \item We insert a single unique non-zero into $C$.
    \item We query $C$ and record whether or not the query succeeded.
    \item We repeat steps $2$-$3$ until the column contains $n$ non-zeroes.
    \item We repeat steps $1$-$4$ for $500$ trials
\end{enumerate}

% There is correlation between our data points across $z$ but not between trials. That is, for a given $z$, each Bernoulli trial is independent. 

Our implementation forgoes the additional depth-1 bucket $b^*_1$. For this reason, we omit the case of $z=2$ from our analysis.

Due to high correlation between $z$ values, we limit our analysis to counting the number of $z$ value-means that are above a given threshold. If a given $z$ value (or, more likely, a region of $z$ values) had a much different probability than other regions, this experiment would still likely catch it. This is because if two non-zero values are highly correlated then their probabilities of success must be very similar. By Bayes Theorem, if $P[A \mid B] \approx 1$ and $P[B \mid A] \approx 1$ then $P[A] \approx P[B]$. This experiment would also catch if xxHash is insufficient for use with \sketchname.

For all values $z$, the mean probability of success is greater than $0.76$. For $99\%$ of the $z$ values, their mean success probability was greater than $0.78$. Additionally, the standard deviation is less than $0.02$ for all $z$.

%$n=2^{24}$, 500 trials, tested every possible number of non-zeros $\forall z \in [n] P[\text{sketch on $z$ non-zeros is good}] \geq 0.78$. 

xxHash, our hash function of choice, provides no proofs of $k$-wise independence or uniformity. Nevertheless, these results indicate xxHash is sufficient for use with \sketchname.
%We experimentally show how many rounds of Boruvka's algorithm it takes \sysname to compute the connected components. We perform this experiment on the data sets from Table \ref{tab:datasets} as well as graphs representing a single unbroken path. For each graph, we ingest and compute the connected components, measuring the number of rounds required.

%The path graphs are randomly generated by permuting a vector of integers. The permutation determines the connectivity; adjacent integers represent adjacent vertices in the path. We compute 100 different path graphs and measure the number of rounds for each.

%For the Table \ref{tab:datasets} we re-ran the ingesting and computation of the connected components 100 times. Each measurement used different random state.
