# Supplementary material for: Exploring the Landscape of Distributed Graph Sketching
Source: arXiv:2410.07518 source file (2024-11-15)
Supplement: Supplementary file 4 [file network_experiment_full.tex]

\section{Network Communication}
\label{app:networkcomm}

\begin{figure}
\centering
\begin{subfigure}{0.45\textwidth}
    \includegraphics[width=\textwidth]{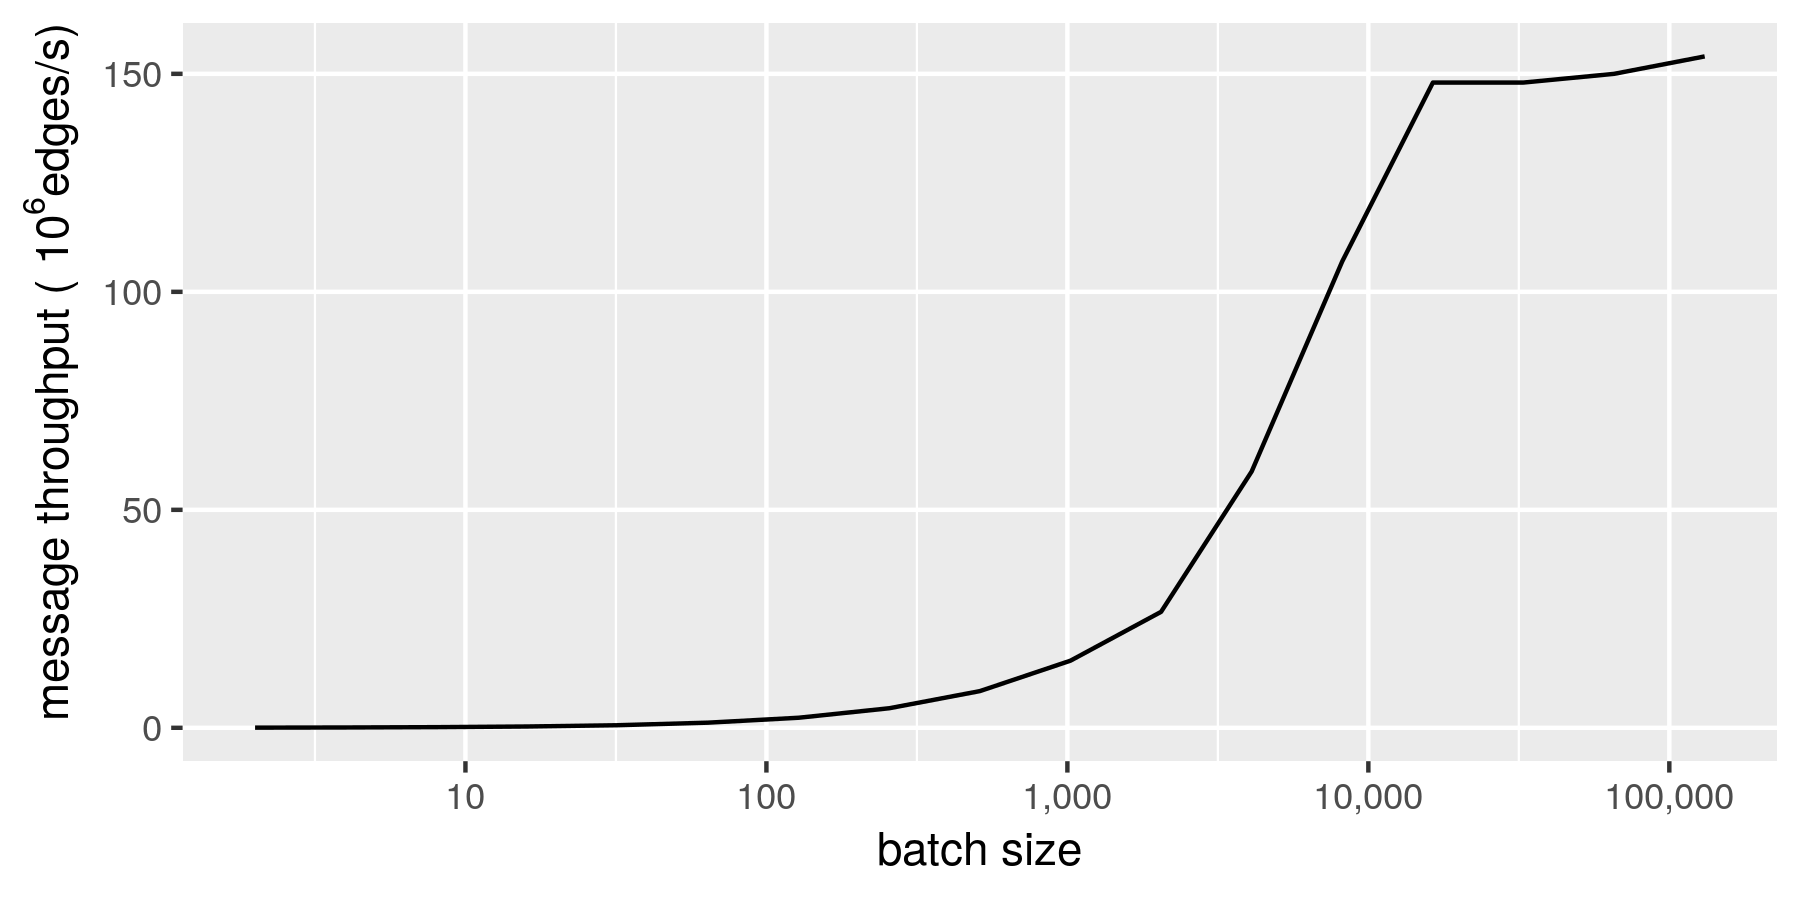}
    \caption{Network message throughput vs batch size.}
    \label{fig:network_throughput}
\end{subfigure}
\hfill
\begin{subfigure}{0.45\textwidth}
    \includegraphics[width=\textwidth]{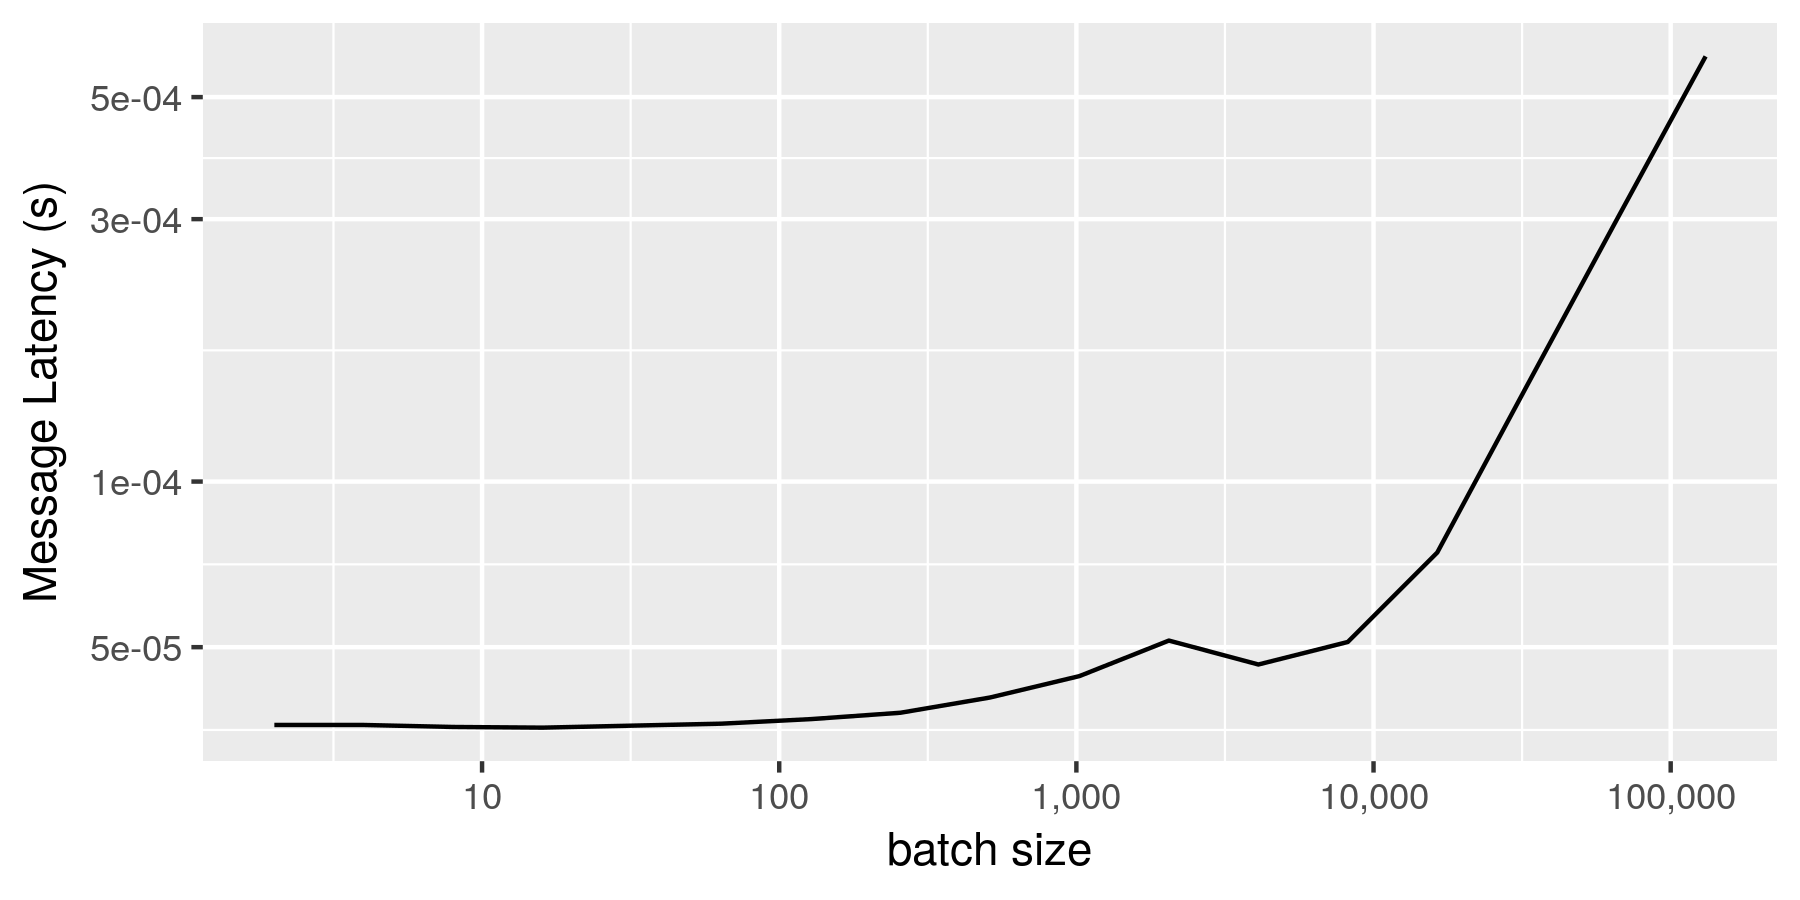}
    \caption{ Network message latency vs batch size.}
    \label{fig:network_latency}
\end{subfigure}

\caption{\sysname's message passing policy maximizes bandwidth use and amortizes away latency costs.}
\label{fig:network}
\end{figure}

Throughout our scaling experiments in Section ~\ref{subsec:scaling} we observe a constant amount of network communication used; approximately $1.6$ times the size of the input stream. Moreover, we demonstrate experimentally that this bandwidth use is near-optimal: Figure~\ref{fig:network} and~\ref{fig:network_throughput} validate our claims that \sysname's vertex-based batches are large enough to amortize the communication costs over the CPU cost of processing sketch updates. Figure~\ref{fig:network_throughput} shows that OpenMPI messages containing vertex-based batches hit the half-bandwidth point when they contain at least several thousand updates. Figure~\ref{fig:network_latency} shows that at this batch size the costs of serializing and sending the message are quite small: the latency is less than $0.1$ millisecond. We configure \sysname to produce vertex-based batches a factor $1.2 \times$ larger than a sketch delta. For a graph on $2^{17}$ vertices, the size of a vertex-based batch is $42$KiB or $10,670$ edge updates. We conclude that \sysname successfully amortizes away the network communication costs, enabling its impressive scaling.
