# Supplementary material for: Exploring the Landscape of Distributed Graph Sketching
Source: arXiv:2410.07518 source file (2024-11-15)
Supplement: Supplementary file 6 [file appendix_old.tex]

\subsection{Prior Work in Connected Components Sketching}
\label{app:alg}
We summarize \algname and \graphzep, respectively Ahn \etal's~\cite{Ahn2012} and Tench \etal's~\cite{graphzeppelin} semi-streaming algorithms for computing a spanning forest (and therefore the connected components) of a graph.  These algorithms have some overlap so for conciseness we describe them in parallel and note where they differ.

For each vertex $v_i$ in $G$, define the \defn{characteristic vector} $\charvec_i$ of $v_i$ to be a 1-dimensional vector indexed by the set of possible edges in $\graph$.  $\charvec_i[(j,k)]$ is only nonzero when $i = j$ or $i = k$ and edge $(j,k) \in \edges$.  That is, $\charvec_i \in \{-1,0,1\}^{\nodesize \choose 2}$ s.t. for all $0 \leq j < k < {\nodesize \choose 2}$: 
$$\charvec_i[(j,k)] = \left\{ \begin{array}{ll}
            1 & \quad i = j \text{ and }(v_j, v_k) \in \edges \\
            -1 & \quad i = k \text{ and }(v_j, v_k) \in \edges \\
            0 & \quad \text{otherwise} 
            
        \end{array}\right\}%\{1$ $if$ $i = j$ $and$ $(v_j, v_k) \in E, -1$ $if$ $i = k$ $and$ $(v_j, v_k) \in E, 0 \text{ otherwise}\}
$$

%The characteristic vector $a_i$ is a 1-dimensional vector indexed by the set of possible edges in $\graph$.  $a_i[(j,k)]$ is only nonzero when $i = j$ or $i = k$ and edge $(j,k) \in \edges$.

These characteristic vectors have an important property that is vital for computing connectivity: For any $S \subset \nodes$, the sum of the characteristic vectors of the vertices in $S$ is a direct encoding of the edges across the cut $(S, \nodes \setminus S$).  That is, let $x = \sum_{v \in S} \charvec_v$ and then % $x\in \{-1,0,1\}^{n \choose 2}$ and 
$|x[(j,k)]| = 1$ iff $(j,k) \in E(S, \nodes \setminus S)$.

%\input{figures/supernode_example}

It is simple to update the characteristic vectors as stream updates arrive. Initialize $\charvec_i = \{0\}^{\nodesize \choose 2}$ for all $i$. For each stream update $s = ((u,v), \Delta)$, set $\charvec_u[u,v] += \Delta$ and $\charvec_v[u,v] += -\Delta$.Using these vectors, we immediately have a (very inefficient) algorithm for computing the connected components from a stream by running Boruvka's algorithm~\cite{boruvka} for finding a spanning forest as follows.  For the first round of the algorithm, from each $a_i$ arbitrarily choose one nonzero entry $(w,y)$ (an edge in $\edges$ s.t. w = i or y = i).  Add $e_i$ to the spanning forest.  For each connected component $C$ in the spanning forest, compute the characteristic vector of $C$: $\charvec_C = \sum_{v\in C} \charvec_v$.  Proceed similarly for the remaining rounds of Boruvka's algorithm: in each round, choose one nonzero entry from the characteristic vector of each connected component and add the corresponding edges to the spanning forest.  Sum the characteristic vectors of the component vertices of the connected components in the spanning forest, and continue until no new merges are possible.  This will take at most $\log(\nodesize)$ rounds.

The key idea to make this a small-space algorithm is to use ``$\ell_0$-sampling''~\cite{l0sketch} to run this version of Boruvka's algorithm by compressing each characteristic vector $\charvec_i$ into a data structure of size $O(\log^2(\nodesize))$ that can return a nonzero entry of $\charvec_i$ with high probability.  For all $\ell_0$ samplers discussed in this paper, $\sketch(\charvec)$ is a vector and adding two sketches is equivalent to adding their vectors elementwise.

\algname uses an $\ell_0$ sampler of Cormode \etal:

\begin{theorem} (Adapted from ~\cite{l0sketch}, Theorem 1):
Given a 2-wise independent hash family $\mathcal{F}$ and an input vector $x \in \mathbb{Z}^n$, there is an $\ell_0$-sampler using $O(\log^2(n))$ space that succeeds with probability at least $1- 1/n^c$ for constant $c$.
\end{theorem}

\graphzep uses \sketchname, an $\ell_0$ sampler that is purpose-built for sketching characteristic vectors and as a result reduces average-case update cost:

\begin{theorem} (Adapted from ~\cite{graphzeppelin}, Theorem 1)
\sketchname is an $\ell_0$ sampler that, for vector $x \in \{-1,0,1\}^n$, has space complexity $O(\log^2(n))$, worst-case update complexity $O(\log^2(n))$, average-case update complexity $O(\log(n))$, and failure probability $O(1/n^c)$ for constant~$c$.
\end{theorem}

For \sysname we choose to use \sketchname for $\ell_0$ sampling because it performs better in practice~\cite{graphzeppelin}.

We denote the $\ell_0$ sketch of a vector $x$ as $\sketch(x)$.  Since the sketch is linear, $\sketch(x) + \sketch(y) = \sketch(x+y)$ for any vectors $x$ and $y$.  This allows us to process stream updates as follows: we maintain a running sum of the sketches of each stream update, which is equivalent to a sketch of the vector defined by the stream. That is, let $\charvec_i^t$ denote $\charvec_i$ after stream prefix $\stream_t$. For the $j$th stream update $\streamelement_j = ((i,x),\Delta)$ we obtain $\sketch(\charvec_i^j) = \sketch(\streamelement_j) + \sketch(\charvec_i^{j-1})$. For each stream update $\streamelement_j$, \algname computes $\sketch(\charvec_i^j)$ as soon as $\streamelement_j$ arrives from the input stream. In contrast, \graphzep inserts $\streamelement_j$ into a \defn{gutter tree} of size $O(\nodesize \log^3(\nodesize))$ that write-efficiently collects updates by endpoint. When $O(\log^3(\nodesize))$ updates have been collected for vertex $i$, $\streamelement_j$ and all other collected updates for vertex $i$ are added to $\sketch(\charvec_i)$. The gutter tree allows stream ingestion to be done I/O optimally when the gutter tree and sketches are stored on disk; we omit the details here.

Linearity also allows Ahn \etal to emulate the merging step of Boruvka's algorithm by summing the sketches of all vertices in each connected component.  They require $\log(\nodesize)$ independent $\ell_0$ sketches for each $v \in \nodes$, one for each round\footnote{Ahn \etal~\cite{Ahn2012} the authors note that adaptivity concerns require the use of new sketches for each round of Boruvka's algorithm.}, so the size of the sketch data structure for each vertex is $O(\log^3(\nodesize))$.  We refer to the sketch data structure for each vertex as a \defn{vertex sketch} and each of its $\log(\nodesize)$ $\ell_0$-subsketches as \sketchname{}s. Since \graphzep is designed to run efficiently out-of-core, it modifies this iterated vertex merging process to be write-optimal~\cite{graphzeppelin}; we omit the details here because \sysname does not use this technique.

The total size of the entire sketch data structure for either algorithm is $O(\nodesize \log^3(\nodesize))$. \graphzep's gutter tree structure also has size $O(\nodesize \log^3(\nodesize))$. Recent work ~\cite{nelson2019optimal} has shown that this space is optimal. Because their $\ell_0$ sketch algorithms are randomized and can sometimes fail, the connectivity algorithm may also fail (subject to the choice of randomness used for the sketches). However, they show that these algorithms succeed with high probability: \ie they fail to return the correct answer with probability at most $1/\nodesize^c$ for some constant $c\geq1$.

\iffalse
\subsection{Proof of Theorem~\ref{thm:queries}}
\label{app:pf}
\begin{proof}
In the worst case, the input stream sends $O(\alpha\gamma\sketchsize\nodesize)$ edge updates such that each vertex $u \in \nodes$ is an endpoint of exactly $\alpha\gamma\sketchsize$ of these edges. Then it issues a connectivity query. At this point, each leaf (which has size $\alpha\sketchsize$ is exactly a $\gamma$-fraction full, and so sends the contents of each leaf as a vertex-based batch to a distributed worker. The worker responds with a sketch delta of size $\sketchsize$, so the average communication induced per edge update is $O(1\alpha\gamma)$.

Note that no query can induce more communication that this - if any leaf buffer is less than a $\gamma$-fraction full, the updates it contains are processed locally and incur no communication. If any leaf buffer is more than a $\gamma$-fraction full, the average communication per update in that buffer is lower (since the sketch delta is always a fixed size).

If the input stream alternates sending $O(\alpha\gamma\sketchsize\nodesize)$ edge updates as above and issuing connectivity queries, the average communication cost per stream update is $O(1\alpha\gamma)$, regardless of stream length.
\end{proof}

\subsection{\dsuname Design}
\label{app:dsu}
\dsuname consists of a union-find data structure encoding the connected components of the spanning forest, and a hash table containing the edges of the spanning forest. Both of these data structures are compact: they require $O(\nodesize)$ space. After the query $q$, when edge update $e = (u,v)$ arrives from the input stream, in addition to inserting $e$ into the \treename, \sysname also uses $e$ to update \dsuname: if $e$ is an edge insertion and $u$ and $v$ are not in the same connected component, it merges their components in \dsuname's union find in $O(\alpha(\nodesize)$ time, where $\alpha$ is the inverse Ackerman function~\cite{ackermann}. It also adds $e$ to the hash table in $O(1)$ expected time. 

If a second query $q'$ is issued later, \sysname can use \dsuname rather than recompute graph connectivity from scratch, which would take $O(\nodesize \log^3(\nodesize))$ time. For global connectivity queries, \sysname returns \dsuname's hash table in $O(\nodesize)$ time and for batched reachability queries it uses \dsuname's union-find data structure to compute reachability for each of the $k$ vertex pairs in $O(k\alpha(\nodesize))$ time. We demonstrate experimentally in Section~\ref{subsec:queryex} that answering queries using \dsuname is several orders of magnitude faster than the sketch Boruvka algorithm.

However, \dsuname can be rendered useless by subsequent edge updates after query $q$. If one of the edges $e = (u,v)$ in \dsuname's spanning forest is deleted, \dsuname does not retain enough information to determine whether or not vertices $u$ and $v$ are still connected and, if they are, to find a replacement edge. Recovering this information is only possible by running the sketch Boruvka algorithm. When a spanning forest edge is deleted in this way, we say that \dsuname has become \defn{invalid} meaning it is no longer useful for answering connectivity queries. While \sysname maintains a valid \dsuname, as each edge update $e = (u,v)$ arrives if $e$ is a deletion \sysname checks whether or not $e$ is in \dsuname's hash table. If it is, \sysname discards \dsuname as invalid. In the worst case, an adversarial input stream would render \dsuname invalid immediately after each query by deleting a key edge but this behavior is pathological and, as we show in Section~\ref{subsec:scaling}, unlikely to occur in real data streams. For practical data streams it is more likely that \dsuname remains valid for a while after a query, during which time subsequent queries can be answered very quickly.  \dsuname will only eventually become invalid.

Using \dsuname introduces a performance tradeoff: maintaining \dsuname on the main node as stream updates arrive increases the memory access load on the main node, which is already the system's main bottleneck. As a result, maintaining a valid \dsuname moderately reduces \sysname's ingestion rate, as we show in Section~\ref{subsec:queryex}. However, while \dsuname is valid, it reduces query latency by multiple orders of magnitude. If \sysname is running on a workload where queries are frequent or arrive in bursts, using \dsuname will likely give the best performance. On workloads where queries are rare or far apart, \dsuname is unlikely to remain valid between queries and so using \sysname without it gives the best performance. We leave this as a configuration option to the user.

\subsection{\sysname Implementation Details}
\label{app:imp}
\paragraph{Distributed Communication via MPI.}
The main node uses a pool of \defn{Work Distributor} threads to distribute vertex-based batches to worker nodes using MPI\_Issend(), a non-blocking synchronous send. Each Work Distributor is responsible for a set of worker nodes\footnote{Note that there may be many worker nodes per physical machine.}. Once the Work Distributor has sent out batches to each of its workers it waits for sketch deltas to arrive from one worker and then applies the sketch deltas to the associated graph nodes' sketches and sends the worker a new set of batches to process. Using a non-blocking call allows the Work Distributor to prepare new sets of batches for sending to the workers while they are performing sketch updates. The synchronous send keeps OpenMPI from buffering the send locally to ensure RAM bandwidth is not adversely affected.

\paragraph{\Treename.}
The \treename is thread-safe and many \defn{Graph Insertion} threads perform insertions of edge updates into the tree in parallel. Each thread maintains its own copy of the first three levels of the tree, so that synchronization between Graph Insertion threads is rare. When a thread fills up a leaf, it swaps an extra empty leaf with the full leaf  in $O(1)$ time and buffers the full leaf until the thread is ready to move a collection of leaves into the Work Queue. Usually this occurs when a large enough number of leaves are ready or when all updates are forced out of the \treename. When moving updates into the Work Queue the Graph Insertion thread may be blocked if the queue is full, but other Graph Insertion threads will be able to continue moving updates in the meantime.

To avoid the performance detriments of cascading flushes, in which a flush often triggers a flush of one of its children, we implement optimizations inspired by the work in~\cite{BenderDaFa20Flushing}. Specifically, we double the size of our leaves at each level of the tree. This doubling means that, in expectation, when we flush a level one leaf we flush $0.5$ level two leaves, $0.25$ level three leaves, etc. This dramatically improves the latency of each \treename insertion as we no longer expect to traverse an entire root-to-leaf path. 
Additionally, to prevent many leaves from simultaneously filling up and flushing in a burst, we randomize when each leaf's first flush occurs. Each leaf has a randomized fullness parameter $f \in [0.75, 1]$; each leaf's first flush occurs when the leaf reaches $f$ full. Subsequent flushes occur when the leaf is full.

We chose the parameters of the \treename to balance insertion performance and memory footprint.
The first level of the tree consists of 8 leaves each with a 8KB buffer size and a fan-out of 16. At each subsequent level the buffer size and fan-out are both doubled.

\paragraph{Work Queue.}
When data is sent over the network by a Work Distributor, many batches are sent at once in a set so that the message is sufficiently large that network latency costs do not dominate the workload (see Section~\ref{subsec:scaling}. As such, each element in the Work Queue is actually itself a collection of up to $b$ update batches, for some constant $b$. A Work Distributor thread querying for data from the Work Queue will receive up to $b$ batches with a single pop operation. We set $b = 8$ as a default.

Threads interacting with the Work Queue only need to hold locks for a constant amount of time, allowing us to achieve a high degree of parallelism. This is because both push and pop only perform pointer swapping within their critical regions to move around data. The Work Queue uses two linked lists and two mutexes/condition variables to synchronize Graph Insertion and Work Distributor threads. The first of these is a free list consisting of empty Work Queue elements, and the second is a consumer list that holds Work Queue elements that are ready for processing.

To perform a push operation, a Graph Insertion thread first grabs the free list lock and if necessary waits for the free list to be non-empty. Once these conditions are satisfied, the thread swaps the set of empty batches in the Work Queue element with the full batches it wishes to add to the queue, an operation which takes $O(1)$ time. This now populated Work Queue element is added to the end of the consumer list once the Graph Insertion thread acquires the consumer list lock.

Work Distributor threads pop data from the Work Queue by first acquiring the consumer list lock and waiting for the consumer list to be non-empty. 
Once these conditions are met, the Work Distributor pulls a Work Queue element containing batches from the consumer list, serializes the batches, and sends the batches over the network to a worker node to be processed into sketch deltas. 
After serialization is complete and the Work Distributor has locked the free list, the Work Queue element is added back into the free list.

\paragraph{Receiving and applying sketch deltas.}
Before waiting to receive sketch deltas from the workers, a Work Distributor ensures that it has sent 2 sets of batches to each of its worker nodes. Sending 2 sets to each worker allows us to pipeline; that is, while the Work Distributor performs the work of applying the sketch deltas, the worker node is able to simultaneously construct the next set of sketch deltas. The worker node is also able to immediately start work on the next batch.

When the Work Distributor thread is ready to apply sketch deltas it calls MPI\_Recv() to receive a set of sketch deltas from one of its worker nodes. The message is first de-serialized into sketch deltas and then merged with the associated vertex sketches. As we note in Section~\ref{subsec:bandwidth_ingest}, a sketch delta for vertex $u$ is merged with the vertex sketch of $u$ on the main node by bitwise XORing them together. This has comparable performance to a sequential scan over the vertex sketch, making it very fast in practice.

Merging a sketch delta requires locking the corresponding vertex sketch as many threads may attempt mutate this same vertex sketch simultaneously. To do so in a thread unsafe manner could result in an incorrect final sketch state. Fortunately, most sketch deltas are bound for unique nodes and as we note above the critical section is very small. As such, merging sketch deltas is a low order term for stream update processing and can be efficiently performed on the main node.

\subsection{Additional Evaluation Details}
\paragraph{Communication Cost Experiment Details.}
\label{app:comm}
\input{figures/scaling_comm}
Figure~\ref{fig:scaling_comm} experimentally validates Theorem~\ref{thm:ingest} which states that the total network bandwidth \sysname consumes is a small constant fraction larger than that required to read in the input stream.  We see that regardless of the number of worker nodes in use, the network bandwidth used stays essentially constant.

\paragraph{Expanded Scaling Evaluation}
\label{app:scale}
\input{figures/speeds}

Table~\ref{tab:speeds} summarizes \sysname's stream ingestion rate using 2560 worker threads on a variety of synthetic and real-world datasets. It also notes how much network communication is used for each stream as a factor of the input stream size. 
%As with kron17, we concatenate these streams with themselves 10 times \evan{The exact number is actually 7. Don't know if it matters or not though.} to reduce noise from measurement and startup overheads. 
Its ingestion rate is very high on dense graph streams and on google-plus. It is lower on p2p-gnutella and rec-amazon because these datasets are so sparse that by the end of the stream, \sysname's leaf gutters are almost all emptier than the $4\%$ fullness threshold and so most update processing occurs on the main node. For all streams except google-plus the total communication used by \sysname is less than a factor 3 larger than the communication required to recieve the input stream. For google-plus, the graph dataset is sparse enough that most leaf gutters are slightly more than $4\%$ full at the end of the stream, meaning that most vertex-based batches will be processed remotely incurring an additional $1/\gamma = 25$-factor increase in network communication in the worst case (per Theorem~\ref{thm:queries}). We only observe roughly a factor 3 increase in network communication in this case, and this is the largest communication increase we observed on a variety of real-world graph datasets we tested.

\paragraph{RAM bandwidth Comparison Details}
\label{app:bandwidth}
We contextualize the ingestion rate results given in Section~\ref{subsec:scaling} by measuring the (c5n.18xlarge) main node's multi-threaded sequential RAM bandwidth (in addition to its multi-threaded random access RAM bandwidth). We use a widely available benchmarking tool, sysbench~\cite{sysbench}, to measure RAM bandwidth. To measure sequential bandwidth, we use the default sysbench settings (1KiB blocks written, 100GB total writes, sequential  global writes) with threads equal to the total number of hardware threads. We find our main node's sequential RAM saturation point is 36 threads, where it achieves a bandwidth of $12700$ MiB/sec ($12.4$ GiB/sec). To measure random access bandwidth, we change the sysbench settings to support smaller blocks (128 bytes) and random writes instead of sequential. We find our main node's random access RAM saturation point to be 36 threads, where it achieves a bandwidth of $759$ MiB/sec.  Since graph stream updates are 9 bytes, we expect this random access bandwidth estimate to be an upper bound -- it is likely to be even slower when making random writes for single stream updates.
We also determined the sequential RAM bandwidth of the r6i.16xlarge instance used in the scaling experiment above to be $19200$ MiB/sec($18.8$ GiB) and random access RAM bandwidth of $991$ MiB/sec.

\sysname's 183 million update/sec ingestion rate on kron17 translates to a stream bandwidth of $195\cdot10^6\cdot9$B\,$ \approx1.63$GiB/second, more than twice as fast as random access RAM bandwidth. Further, \sysname's ingestion bandwidth is roughly one-eighth of sequential RAM bandwidth, the theoretical upper bound for any system that receives the input stream at a main node.

\paragraph{Query Latency Breakdown.}
\label{app:breakdown}
\input{figures/query}
We analyze \sysname's query latency on an extended kron17 stream by issuing global connectivity queries periodically and recording (1) the time to flush the cache-optimizing gutter tree and update the graph sketch and (2) to perform Boruvka's algorithm using the graph sketch. The sum of these times is the total query latency, though only the Boruvka computation is additional work induced by the query; the flushing work would have happened anyway as part of stream ingestion even if the query was never issued. Figure~\ref{fig:query} summarizes the results of this experiment: flushing accounts for the majority of the query latency, while Boruvka's algorithm takes roughly half a second. During this experiment, \sysname used $3.4$ times more communication than was required to receive the input stream.


\paragraph{Correctness Experiment Details.}
\label{app:correct}
Like \algname~\cite{Ahn2012} and \graphzep~\cite{graphzeppelin}, \sysname's linear sketching techniques are randomized. The connectivity algorithm may return an incorrect answer (or no answer at all) with probability at most $1/\nodesize^c$ for some constant $c\geq1$. To verify that this small chance of failure is unobservable in practice, we checked the results of 1000 connectivity queries for correctness each on the kron17, p2p-gnutella, rec-amazon, and google-plus datasets. No failures were ever observed, supporting the conclusion that \sysname reliably gives correct answers of graph streams regardless of size or density.

\paragraph{Spark GraphX Comparison Details.}
\label{app:spark}

\input{figures/spark}

Using 16 worker nodes, we ran GraphX's~\cite{gonzalez2014graphx} distributed connected components algorithm on kron13, kron15, and kron16. Since GraphX does not support dynamic or streaming graph computation, we ran it on the static version of these graphs instead. We loaded each graph onto the main node and converted it into the GraphFrame format, and then GraphX's distributed connected component algorithm. The results of these experiments are summarized in Table~\ref{tab:spark}. GraphX is takes much more time to process these dense graph datasets than \sysname, even though it is processing a static graph instead of a graph stream. Spark timed out GraphX's connected components algorithm after more than an hour of computation on kron16. In addition, GraphX's communication cost sometimes appears to be quite high: for its incomplete run on kron16, it already used 11 times the size of the graph in network communication and presumably would use more if it had completed its computation.
\fi
